# Supplementary material for: On Algorithmic Decision Procedures in Emergency Response Systems in Smart and Connected Communities
Source: arXiv:2001.07362 source file (2020-03-12)
Supplement: Supplementary file 1 [file appendix.tex]

\newpage
\section{Appendix}

\subsection{Rebuttal}

\subsubsection{Review $#$1}

\subsubsection{Review $#$2}

\subsubsection{Review $#$2}
